# Supplementary material for: Measuring collective diffusion properties by counting particles in boxes
Source: arXiv:2412.14122 ancillary file (2025-03-25)
Supplement: Supplementary file 1 [file supplementary_info.pdf]

# Supplementary Information

Measuring collective diffusion properties by counting particles in boxes

A. Carter, E. K. R. Mackay, B. Sprinkle, A. Thorneywork, S. Marbach

December 17, 2024

## Supplementary Discussion

**1 Supplementary analysis** **2**
1.1 Countoscope rescaling in the dilute regime . . . . . . . . . . 2
1.2 Countoscope plateau value . . . . . . . . . . 3
1.3 Effect of simulation box size on $D(L)$, $D(k)$ . . . . . . . . . . 5
1.4 $f(k,t)$ behaviour at short and long times . . . . . . . . . . 6
1.5 $f(k,t)$ short time divergence . . . . . . . . . . 7

# 1 Supplementary analysis

## 1.1 Countoscope rescaling in the dilute regime

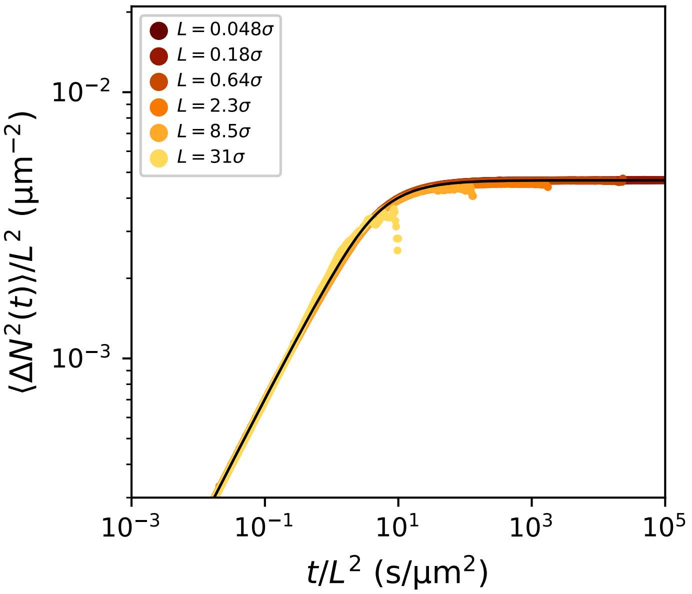


**Figure S1:** At $\phi = 0.02$, the data rescales onto itself for all box sizes. The black line corresponds with the theory Eq. (3) in the main text. Points correspond to experimental data. This rescaling also illustrates that the plateau value corresponds to two times the mean number of particles in a box in the dilute regime, mathematically $\mathrm{Var}(N) = \langle N \rangle$.

## 1.2 Countoscope plateau value

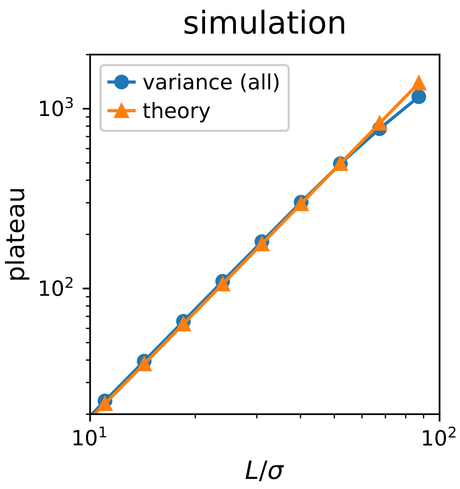


**Figure S2:** Plateau values against box size for simulations and experiments. The plateau is defined as $2\mathrm{Var}(N)$. It is either measured by computing $\mathrm{Var}(N)$ over all boxes and all times (blue) or calculated via the expression of $C_N(t=0) = \mathrm{Var}(N)$ of Eq. (12) of the main text (orange). Packing fraction is $\phi = 0.11$. The deviation of the variance from it's theoretical value for experiments shows that we do not have enough data to properly resolve the variance at large $L$, a problem that is less significant for the simulation.

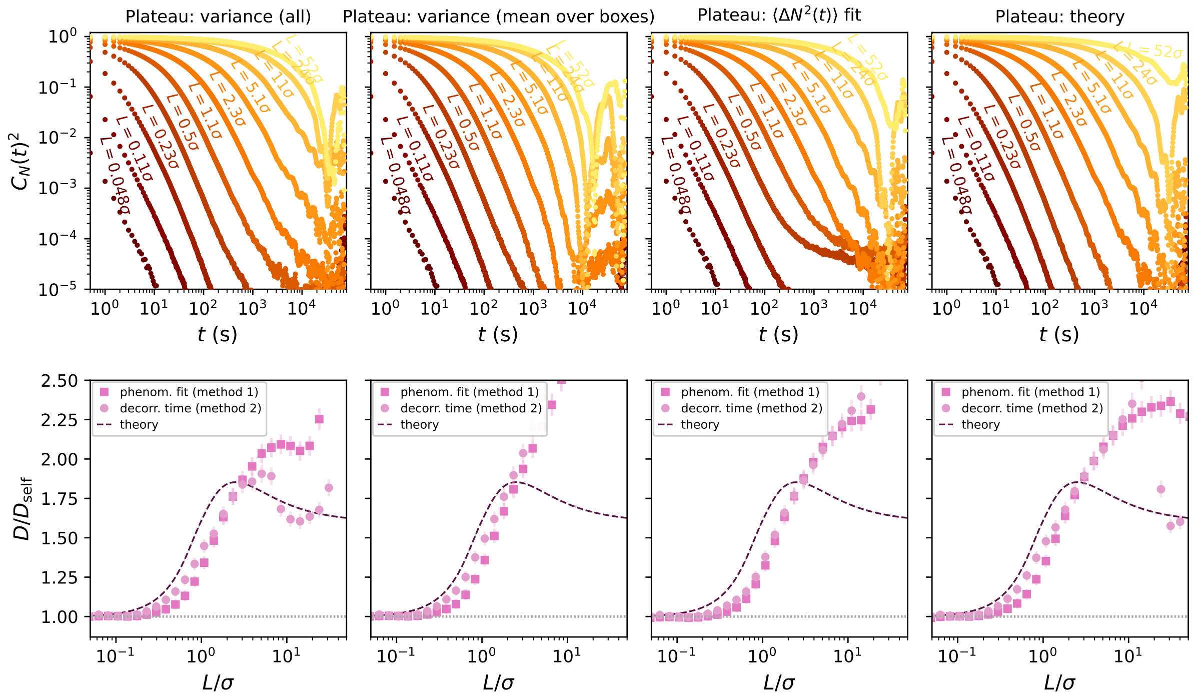


**Figure S3:** Curves of $C_N(t)^2$ and $D(L)$ shown for different sources of the plateau value, for the experimental data at $\phi = 0.11$. "Variance (all)" is the variance of $N(t)$, calculated over all boxes and times. "Variance (mean over boxes)" is the variance over time for each box, averaged over all boxes. "$\langle \Delta N^2(t) \rangle$ fit" is a fit to Eq. 6 with $\mathrm{Var}(N)$ and $D(L)$ free parameters. Plateau: "theory" is given by $= 2\mathrm{Var}(N) = 2C_N(t=0)$ of Eq. (12) of the main text.

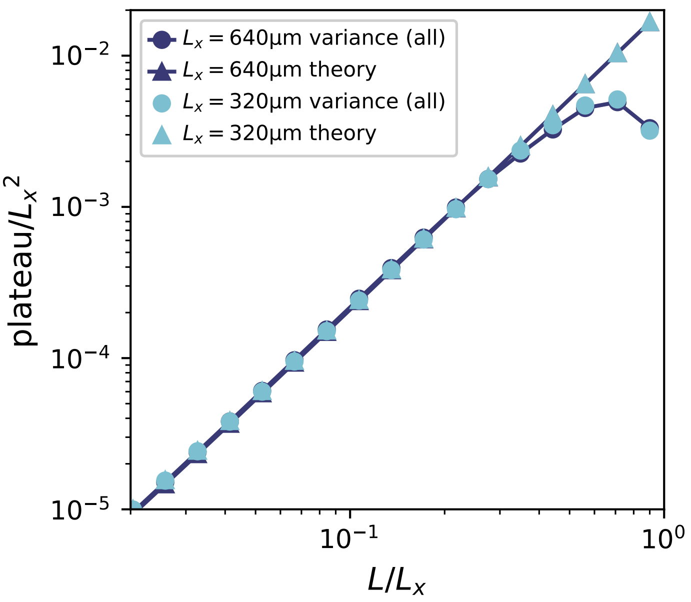


**Figure S4:** Effect of periodic boundary conditions in simulations on Countoscope plateau determination. The plot is similar to Fig. S2: the plateau is defined as 2Var($N$). It is either measured by computing Var($N$) over all boxes and all times (circles) or calculated via the expression of $C_N(t = 0) = \mathrm{Var}(N)$ of Eq. (12) of the main text (triangles). Packing fraction is $\phi = 0.11$. The different colours indicate different sizes $L_x = L_y$ of the periodic simulation box size. The circles, respectively the triangles, perfectly overlap one another. The variance (circles) underestimates the theoretical plateau value (triangles) for boxes $L \gtrsim 0.3L_x$, regardless of the magnitude of the simulation box size. This is an effect of periodic boundary conditions that prevent fluctuations are large spatial scales.

## 1.3 Effect of simulation box size on $D(L)$, $D(k)$

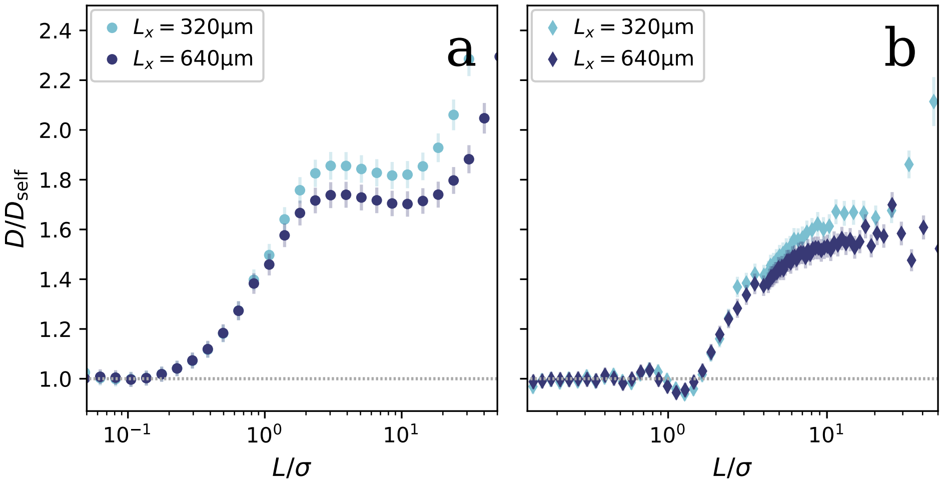


**Figure S5:** $D(L)$ from (a) decorrelation timescale $T(L)$ of number fluctuations (method 2) and (b) dynamic structure factor for two different sizes $L_x$ of the periodic simulation box. Increasing the box size clearly shows that large scale $D(L)$ is reduced in larger simulation domains. In addition, the divergence seen in (a) shifts from $L \gtrsim 10\sigma$ for $L_x = 320$ $\mu$m to $L \gtrsim 10\sigma$ for $L_x = 640$ $\mu$m.

### 1.4 $f(k,t)$ behaviour at short and long times

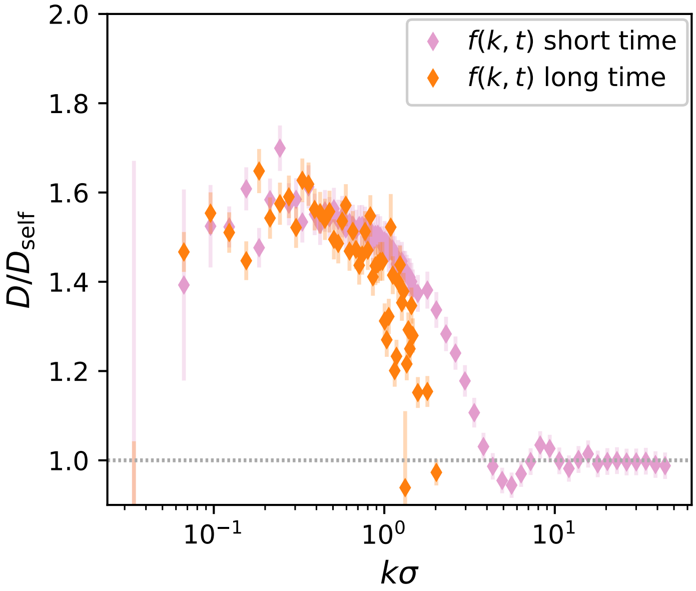


**Figure S6:** $D(k)$ from $f(k,t)$ at short and long times, from simulation, at $\phi = 0.11$. The dynamic structure factor decays too quickly for us to be able to extract long-time information at large $k$ values. Short-time data is obtained from inverting the first (non-zero) point of $f(k,t)$, as described in the main text. Long-time data is obtained from fitting to Eq. 10 for $100 < t < 1000$.

## 1.5 $f(k,t)$ short time divergence

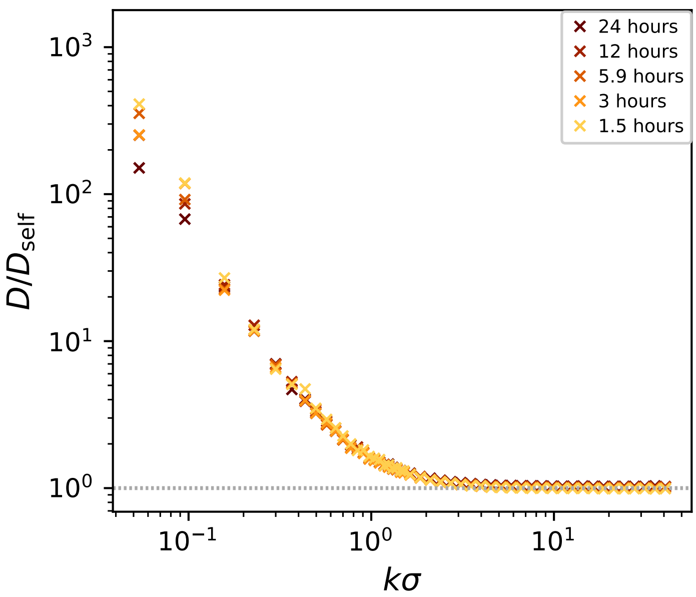


**Figure S7:** Experimental data of $D(k)$ at $\phi = 0.02$. The divergent behaviour of $D(k)$ at small $k$ is independent of movie length.

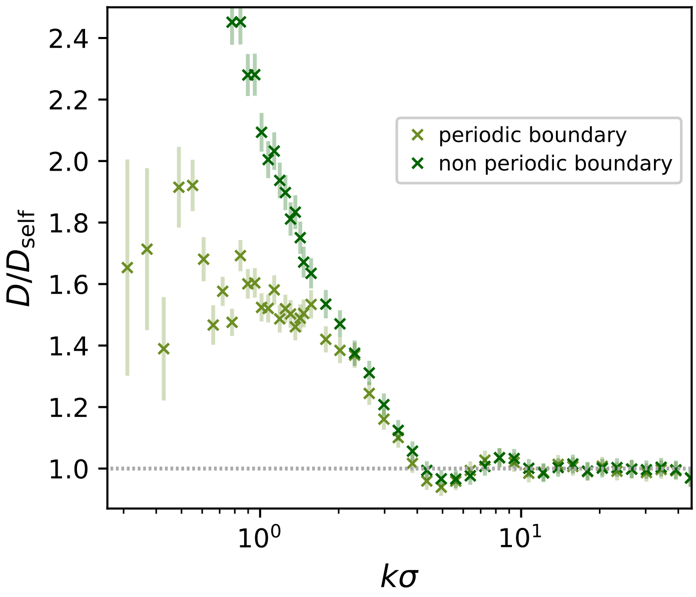


**Figure S8:** $D(k)$ from $f(k,t)$ from data with periodic and non periodic boundary conditions at high density for experimental data ($\phi = 0.11$). Similarly to the low-density case, a divergence is seen for small $k$ (large length scales) when the data is not periodic.
